# Supplementary material for: Mechanism of chain collapse of strongly charged polyelectrolytes
Source: arXiv:1606.02095 source file (2016-06-07)
Supplement: Supplementary file 1 [file suppInfo.pdf]

*Supplementary material for*

# Mechanism of chain collapse of strongly charged polyelectrolytes

**Anvy Moly Tom***, **Satyavani Vemparala***, **R. Rajesh*** and **Nikolai V. Brilliantov**†

* *The Institute of Mathematical Sciences, C.I.T. Campus, Taramani, Chennai 600113, India*

† *Department of Mathematics, University of Leicester, Leicester LE1 7RH, United Kingdom*

## 1 Robustness of the scaling for the gyration radius

We have verified that the exponents and associated features seen in Fig. 1 of the main text are robust and independent of the details of the interaction potential and solvent model. We simulated two other systems for the good solvent conditions. For the first system we use the Lennard-Jones (LJ) potential which includes the attractive part ($r_c = 2.5\sigma$, $\epsilon = 0.25\,\epsilon_0$) for monomer-monomer pairs and purely repulsive interactions ($r_c = 1.0\sigma$, $\epsilon = \epsilon_0$) for all other pairs. Note that in spite of the presence of the attractive part the LJ potential, the second virial coefficient is positive for this value of $\epsilon$, at temperature $k_BT/\epsilon_0 = 1$, which corresponds to a good solvent. The results are shown in Fig. S1.

For the second system we perform simulation of PE chain in the presence of explicit solvent molecules. We use the attractive interactions between monomers and solvent pairs ($r_c = 2.5\sigma$, $\epsilon = \epsilon_0$) and repulsive for all other pairs, see Fig. S2. We also confirm that the results are independent of the length of the chain $N$ for all values of $\ell_B$, see Fig. S3.

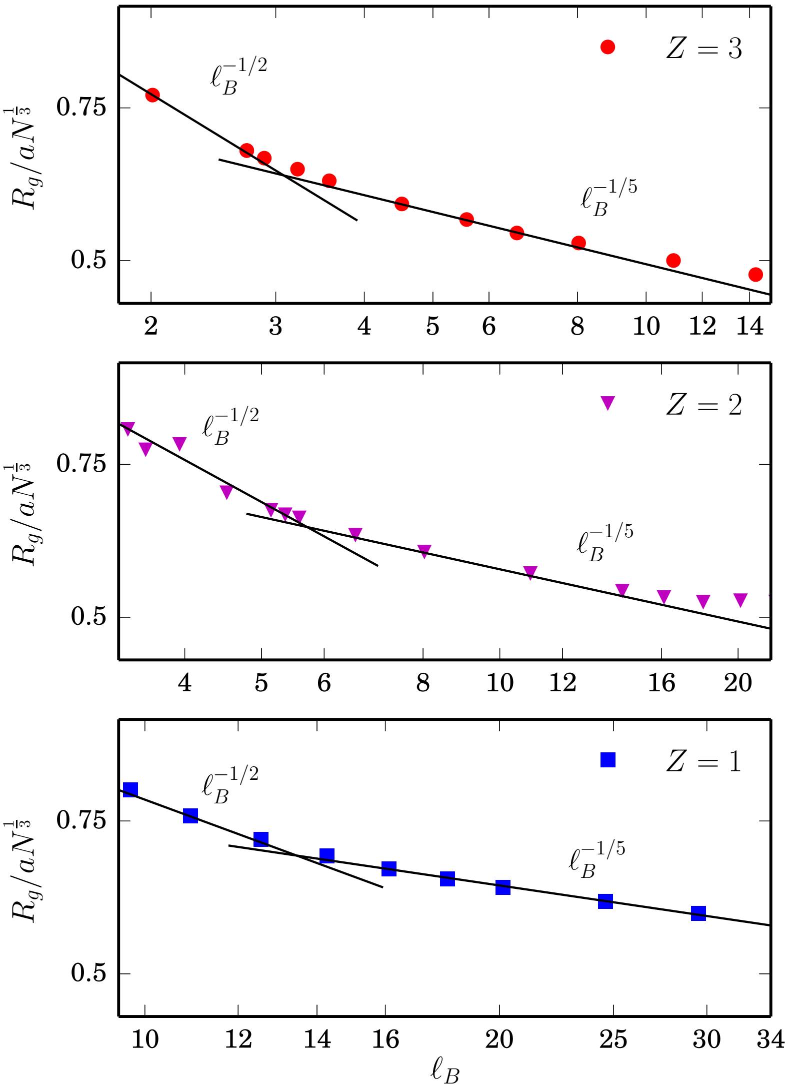


S1: The variation of the gyration radius $R_g$ with $\ell_B$ for a system with LJ interactions being attractive ($r_c = 2.5\sigma$, $\epsilon = 0.25\,\epsilon_0$) for monomer-monomer pairs and purely repulsive ($r_c = 1.0\sigma$, $\epsilon = \epsilon_0$) for all other pairs and PE chain of length $N_m = 204$. The temperature of the system is kept at $k_BT/\epsilon_0 = 1$.

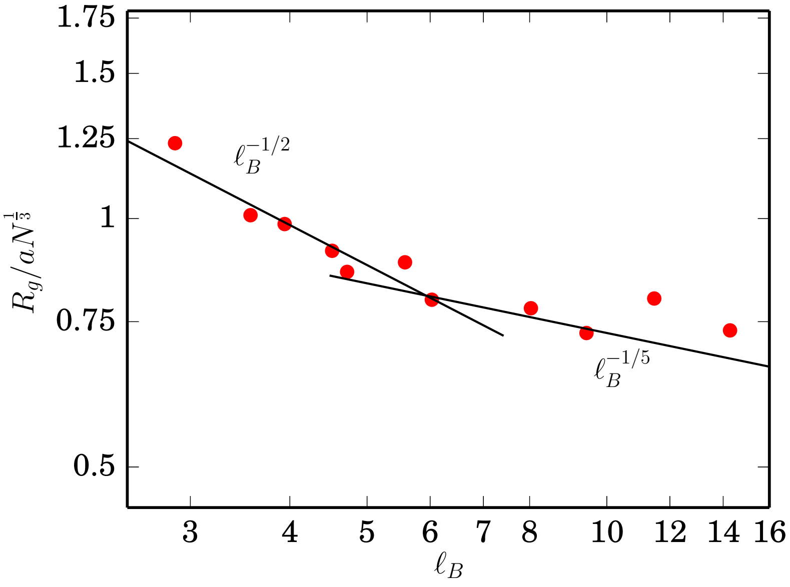


S2: The variation of the gyration radius $R_g$ with $\ell_B$ for a system containing explicit solvent molecules with LJ interaction being attractive ($r_c = 2.5\sigma$, $\epsilon = \epsilon_0$) for monomer and solvent particles pairs and purely repulsive ($r_c = 1.0\sigma$, $\epsilon = \epsilon_0$) for all other pairs. The data are for the system with $Z = 3$. The PE chain of length $N_m = 99$ and number of solvent molecules $N_s = 10000$. The temperature of the system is kept at $k_BT/\epsilon_0 = 1$.

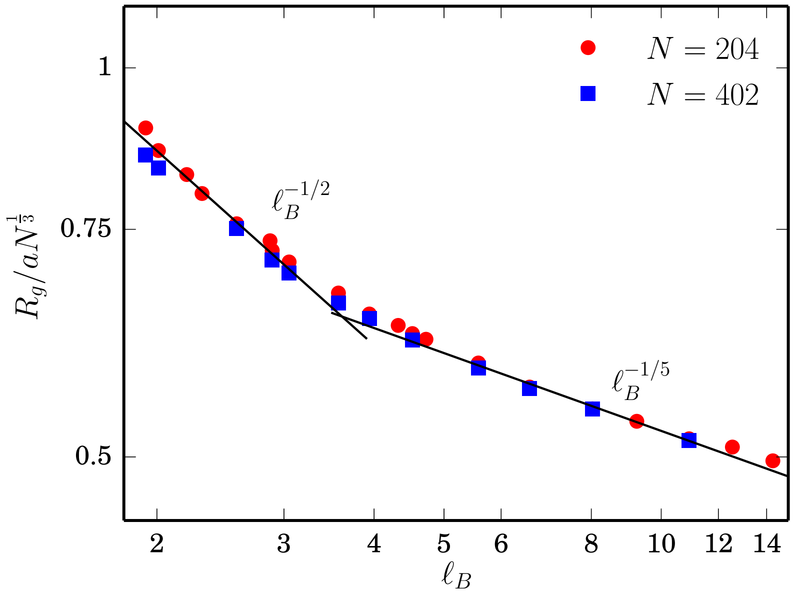


S3: The variation of the gyration radius $R_g$ with $\ell_B$ for different chain lengths. The data are for a system with trivalent counterions and LJ interaction being purely repulsive ($r_c = 1.0\sigma$, $\epsilon = \epsilon_0$) for all pairs. The temperature of the system is kept at $k_BT/\epsilon_0 = 1$.

# 2 Renormalization of the virial coefficients

We consider the contribution to the free energy of the system from the volume interactions between monomers and counterions and between the counterions themselves. We assume that the PE is in a collapsed state, so that almost all counterions $N_c$ are located within the gyration volume $V_g = (4\pi/3)R_g^3$. Then the part of the free energy, corresponding to the volume interactions of the counterions may be written as

$$F_{\rm vol.cc} = \left(\frac{1}{2}B_{cc}\rho_c^2 + \frac{1}{6}C_{cc}\rho_c^3\right)V_g \qquad (1)$$

where $B_{cc}$ and $C_{cc}$ are respectively the second and third virial coefficients that describe counterion-counterion interactions and $\rho_c = N_c/V_g = N/ZV_g$ is the average density of counterions within the gyration volume. Similarly, the part of the free energy, corresponding to the volume interactions between counterions and chain monomers reads,

$$F_{\rm vol.cm} = \left(B_{cm}\rho_c\rho_m + \frac{1}{2}C_{cc\,m}\rho_c^2\rho_m + \frac{1}{2}C_{c\,mm}\rho_c\rho_m^2\right)V_g, \qquad (2)$$

where $B_{cm}$, $C_{cc\,m}$ and $C_{c\,mm}$ are respectively second and third virial coefficients for monomer-counterion volume interactions and $\rho_m = N/V_g$ is the average density of monomers within the gyration volume. Finally, the part of the free energy that refers to the monomer-monomer volume interactions has the form [see Eq. (7) of the main text]:

$$F_{\rm vol} \equiv F_{\rm vol.mm} = \left(\frac{1}{2}B\rho_m^2 + \frac{1}{6}C\rho_m^3\right)V_g. \qquad (3)$$

Using the above equations one can write, after some algebra, the free energy of the system, related to all volume interactions as

$$\begin{aligned} F_{\rm vol.tot} &= F_{\rm vol.cc} + F_{\rm vol.cm} + F_{\rm vol.mm} \qquad (4) \\ &= \frac{\tilde{B}}{N^{1/2}\alpha^3} + \frac{\tilde{C}}{N\alpha^6}, \end{aligned}$$

with

$$\begin{aligned} \tilde{B} &= \frac{9\sqrt{6}}{4\pi a^3}\left[B + \frac{2B_{cm}}{Z} + \frac{B_{cc}}{Z^2}\right] \qquad (5) \\ \tilde{C} &= \frac{81}{4\pi^2 a^6}\left[C + \frac{3C_{c\,mm}}{Z} + \frac{3C_{cc\,m}}{Z^2} + \frac{C_{cc}}{Z^3}\right]. \end{aligned}$$

In other words, one can write $F_{\rm vol.tot}$ in the same form as the volume part of the free energy $F_{\rm vol}$ in Eq. (7) or (10), but with the renormalized virial coefficients.

The above equations are the generalization of Eq. (7) of the main text. As it is follows from the above equations, in order to take into account the volume interactions with the counterions for the case of globular state of a PE and complete condensation of counterions, it is sufficient to perform the renormalization of the virial coefficients according to the rule:

$$\begin{aligned} B &\to B + \frac{2B_{cm}}{Z} + \frac{B_{cc}}{Z^2} \\ C &\to C + \frac{3C_{c\,mm}}{Z} + \frac{3C_{cc\,m}}{Z^2} + \frac{C_{cc}}{Z^3}. \end{aligned}$$

For simplicity we keep the same notations for these coefficients as for the coefficients in Eqs. (7) and (10) of the main text.
